# Supplementary material for: Granular solids transmit stress as two-phase composites
Source: arXiv:2306.10581 source file (2023-12-22)
Supplement: Supplementary file 1 [file TwoPhaseGM_SM.pdf]

# Granular solids transmit stress as two-phase composites
# Supplemental material

Raphael Blumenfeld*
*Gonville & Caius College, University of Cambridge, Trinity St., Cambridge CB2 1TA, UK*†
(Dated: August 31, 2023)

PACS numbers:

## I. THE GENERAL SOLUTIONS OF ISOSTATICITY THEORY IN $d = 2$

Following the notation in the main text, the general equations of isostaticity theory (IT) are:

$$\vec{\nabla} \cdot \overline{\overline{\sigma}} = \vec{g}_{ext} \qquad \text{(balance of forces)} \tag{1}$$

$$\overline{\overline{\sigma}} = \overline{\overline{\sigma}}^T \qquad \text{(balance of torques)} \tag{2}$$

$$\overline{\overline{M}} : \overline{\overline{\sigma}} = 0 \qquad \text{(stress} - \text{structure relation)} \ , \tag{3}$$

in which $\overline{\overline{\sigma}}$ is the stress tensor, $g_{ext} = (g_x, g_y)^T$ is an external force field, which includes loading and body forces, and $\overline{\overline{M}}$ a symmetric tensor that describes the chirality of the local fabric structure [1, 2], i.e., a fabric tensor. These equations are presumed coarse-grained to a continuum scale [3]. In $d = 2$, where the tensor $\overline{\overline{B}}$ can be derived directly from the grain-scale structure, these equations reduce to

$$\partial_x \sigma_{xx} + \partial_y \sigma_{xy} = g_x \tag{4}$$

$$\partial_x \sigma_{xy} + \partial_y \sigma_{yy} = g_y \tag{5}$$

$$m_{xx}\sigma_{xx} + 2m_{xy}\sigma_{xy} + m_{yy}\sigma_{yy} = 0 \ , \tag{6}$$

in which $\partial_\alpha \equiv \partial/\partial\alpha$. Briefly, the solutions of isostaticity theory in $d = 2$ are obtained as follows [4, 5]. Firstly, express $\sigma_{yy}$ in term of $\sigma_{xx}$ and $\sigma_{xy}$, using eq. (6),

$$\sigma_{yy} = \frac{-1}{m_{yy}} \left( m_{xx}\sigma_{xx} + 2m_{xy}\sigma_{xy} \right) \ . \tag{7}$$

Defining

$$\vec{u} = (\sigma_{xx}, \sigma_{xy})^T \quad \text{and} \quad \overline{\overline{A}} = \frac{1}{m_{yy}} \begin{pmatrix} 0 & m_{yy} \\ m_{xx} & -2m_{xy} \end{pmatrix} \ , \tag{8}$$

eqs. (4) and (5) can be cast in the form

$$\partial_x \vec{u} + \partial_y \left( \overline{\overline{A}} \cdot \vec{u} \right) = \vec{g}_{ext} \ . \tag{9}$$

The eigenvalues of $\overline{\overline{A}}$ are given by

$$\lambda_{1,2} = \frac{1}{m_{yy}} \left( -m_{xy} \pm \sqrt{-\det\left\{\overline{\overline{M}}\right\}} \right) \ . \tag{10}$$

Since $\det\left\{\overline{\overline{M}}\right\} < 0$ the eigenvalues $\lambda_i$ are distinct and real. This allows us to write eq. (9) in terms of the characteristics

$$\partial_x \vec{\omega} + \overline{\overline{\Lambda}} \cdot \partial_y \vec{\omega} = \vec{h} - \left( \partial_y \overline{\overline{\Lambda}} \right) \vec{\omega} + \overline{\overline{B}} \cdot \vec{\omega} \ , \tag{11}$$

in which $\vec{\omega}$ is a vector of the two characteristic variables, $\omega_i$,

$$\vec{\omega} = \left( \lambda_2\sigma_{xx} - \sigma_{xy}, -\lambda_1\sigma_{xx} + \sigma_{xy} \right)^T \ , \tag{12}$$

$\overline{\overline{\Lambda}} = \begin{pmatrix} \lambda_1 & 0 \\ 0 & \lambda_2 \end{pmatrix}$, $\vec{h} = \frac{(\lambda_2 g_x - g_y, \lambda_1 g_x + g_y)^T}{(\lambda_2 - \lambda_1)}$ is a linear combination of the external forces, and

$$\overline{\overline{B}} = \frac{1}{\lambda_2 - \lambda_1} \begin{pmatrix} \partial_x\lambda_1 + \lambda_1\partial_y\lambda_1 & \partial_x\lambda_2 + \lambda_2\partial_y\lambda_2 \\ -\partial_x\lambda_1 - \lambda_1\partial_y\lambda_1 & -\partial_x\lambda_2 - \lambda_2\partial_y\lambda_2 \end{pmatrix} \ . \tag{13}$$

The solution of eq. (11) for $\vec{\omega}$ can then be converted to resolve the stress components along the characteristic paths:

$$\overline{\overline{\sigma}} = \omega_1 \begin{pmatrix} 1 & \lambda_1 \\ \lambda_1 & \lambda_1^2 \end{pmatrix} + \omega_2 \begin{pmatrix} 1 & \lambda_2 \\ \lambda_2 & \lambda_2^2 \end{pmatrix} \ . \tag{14}$$

For example, given a medium that spans the right half-plane, $x \geq 0$, $-\infty < y, \infty$ and a stress distribution along the boundary at $y = 0$, $\overline{\overline{\sigma}}(x, y = 0)$, the solution at any point $(x, y)$ is found by a superposition of the stresses in (14), each traced along its characteristic path to the values of the characteristic variables, $\omega_i$, on the boundary. For uniform fabric tensors, the characteristic variables at a point inside the medium, $(x, y)$, are

$$\omega_i(x, y) = \omega_i(0, y - \lambda_i x) + \int_0^x h_i(s) ds \quad i = 1, 2 \tag{15}$$

and the stress field at this point is given by the linear combination of eq. (14).

The characteristic variables $\omega_1$ and $\omega_2$ are only coupled in eqs. (11)-(13) by the matrix $\overline{\overline{B}}$. This coupling vanishes when $\overline{\overline{B}}$ is identically zero, which is when the fabric tensor $\overline{\overline{M}}$ is constant across the system, $\vec{\nabla} m_{ij} = 0$. Then the characteristic paths are straight lines and the stress is finite only along them. These paths emanate at gradients $\lambda_i$ from the stress sources. Effects of non-uniformity of this tensor have been discussed, with examples, in previous works [4–6] and include branching, leaking of stresses to secondary chains, stress attenuation, and broadening.

---

*rbb11@cam.ac.uk
†Imperial College, London SW7 2AZ, UK

## II. THE LAYERED PLANAR COMPOSITE

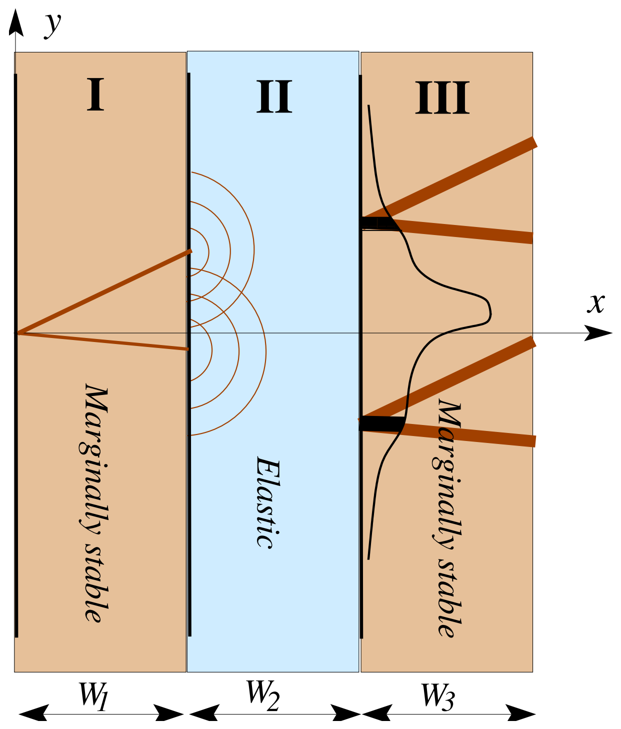


FIG. 1: A stack of alternating marginally rigid and elastic plates. A localised stress is applied at the boundary $x = 0$, generating two stress chains that 'propagate' along two characteristic paths. The chain stresses apply two localised loads on on the strain-free boundary at $x = W_1$, which form the boundary conditions for the elastic plate. The stress response within the elastic plate satisfies the elliptic equations of elasticity theory. The stress response on the strain-free boundary at $x = W_2$ is sketched. Adding another plate of marginally rigid medium at $x = W_2$, the stress solution within it is a superposition of the boundary stress chains, such as the one exemplified in the figure.

The layered system is a simple solvable case of a two-phase system. Consider parallel plates in two dimensions, one of material in the marginally rigid state and the other of elastic medium, as shown in Fig. 1. The thicknesses of these plates are $0 < x_{mr} < W1$ and $W1 < x_e < W2$, respectively, and they extend to $\pm\infty$ in the $y$-direction. For simplicity and illustrative purposes, the structure tensor of the marginally rigid plate is taken to be uniform. A point loading is applied at the origin, $\bar{\bar{\sigma}}(x = 0, y = 0)$. Since the equations are linear in both plates, we can consider only the point loading with the understanding that it is superposed over the uniform stress. Let us chose the following convenient fabric tensor,

$$\bar{\bar{M}} = \begin{pmatrix} 3 & 1 \\ 1 & -1 \end{pmatrix} \;, \tag{16}$$

with $\det\left\{\bar{\bar{M}}\right\} = -4$. Then $\bar{\bar{A}} = \begin{pmatrix} 0 & -1 \\ 3 & -2 \end{pmatrix}$ and its eigenvalues are $\lambda_1 = 3$ and $\lambda_2 = -1$. These are the gradients of the paths shown in Fig. 1. The characteristic variables are:

$$\vec{\omega} = \begin{pmatrix} -\sigma_{xx} - \sigma_{xy} \\ -3\sigma_{xx} + \sigma_{xy} \end{pmatrix} \;. \tag{17}$$

Using (14) we find that

$$\bar{\bar{\sigma}} = \begin{cases} \frac{\sigma_{xx}+\sigma_{xy}}{4} \begin{pmatrix} 1 & 3 \\ 3 & 9 \end{pmatrix} & \text{on path 1} \\ \frac{3\sigma_{xx}-\sigma_{xy}}{4} \begin{pmatrix} 1 & -1 \\ -1 & 1 \end{pmatrix} & \text{on path 2} \\ 0 & \text{elsewhere .} \end{cases} \tag{18}$$

The stress response to the uniform loading on the boundary at $x = 0$ is uniform throughout the first plate and it is evaluated as shown in Fig UniformSol. At each each point within this plate, e.g., point $C$ in the figure, the stress is the superposition of the stress along two characteristic paths emanating from different points along the boundary at $x = 0$, e.g., $A$ and $B$,

$$\begin{aligned} &\bar{\bar{\sigma}}\left(x_C, y_C\right) = \\ &\frac{\sigma_{xx}+\sigma_{xy}}{4} \begin{pmatrix} 1 & 3 \\ 3 & 9 \end{pmatrix} + \frac{3\sigma_{xx}-\sigma_{xy}}{4} \begin{pmatrix} 1 & -1 \\ -1 & 1 \end{pmatrix} \\ &= \begin{pmatrix} \sigma_{xx} & \sigma_{xy} \\ \sigma_{xy} & \sigma_{yy} = 3\sigma_{xx} + 2\sigma_{xy} \end{pmatrix} \;. \end{aligned} \tag{19}$$

Note that the value of $\sigma_{yy}$ is determined by the constitutive stress-structure relation (6).

The response to the loading at the origin produces two point loadings on the boundary at $x = W_1$,

$$\begin{aligned} \bar{\bar{\sigma}}\left(W_1, y\right) = &\frac{\sigma_{xx}+\sigma_{xy}}{4} \begin{pmatrix} 1 & 3 \\ 3 & 9 \end{pmatrix} \delta\left(x - W_1, y - 3W_1\right) \\ + &\frac{3\sigma_{xx}-\sigma_{xy}}{4} \begin{pmatrix} 1 & -1 \\ -1 & 1 \end{pmatrix} \delta\left(x - W_1, y + W_1\right) \;. \end{aligned} \tag{20}$$

These act as two point loadings on the boundary of the elastic plate, giving rise to a stress field in it. The boundary at $x = W_1$ is presumed to allow this stress through by deforming it slightly in a way that satisfies the stress-strain relations in the elastic plate (see main text for discussion of this boundary condition). Then the solution for this field is a standard textbook: $\bar{\bar{\sigma}}^{elas}\left(x > W_1, y\right)$ is derived from the second derivatives of the Airy stress function, which satisfies in this medium the biharmonic equation, $\nabla^4\Phi = 0$.
In turn, this solution generates a more complex stress profile on the boundary at $x = W_2$, which then acts as a continuous boundary loading for the solution in the following marginally rigid plate at $x > W_2$. This boundary is presumed straight, as the following marginally rigid plate requires only the stress on this boundary as a condition. This boundary stress is the superposition of solutions similar to that in the first plate, as sketched in Fig. 1. This analytical solution can be extended to an arbitrary number of alternating marginally

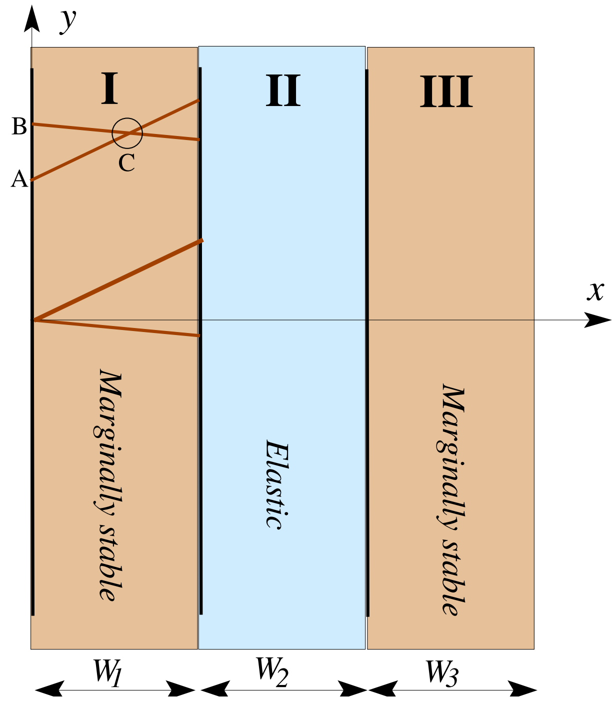


FIG. 2: The stress at point $C$, within the first marginally stable plate is a superposition of the characteristic stresses emanating from points $A$ and $B$ on the boundary at $x = 0$ along the characteristic paths. This stress is uniform throughout this plate except along the characteristic paths emanating from the origin, where an additional point loading is applied.

rigid and elastic plates, but it becomes cumbersome very quickly. To avoid ill-posedness, the assignment of boundary conditions in such an alternating $N$-plate system should be as follows. Let the boundaries be at $x = W_n$, $n = 0, 1, \ldots, N$. The boundaries at $n = 2k$, which transmit stress from elastic to marginally rigid plates, should be regraded rigidly straight. The boundaries at $n = 2k + 1$ should be allowed to allow the stress from the marginally stable to the elastic side by deforming in a manner that matches the linear constitutive stress-strain relations on the elastic side, as discussed in the main text.

[1] R. C. Ball and R. Blumenfeld, Phys. Rev. Lett., **88**, 115505 (2002)
[2] R. Blumenfeld, Phys. Rev. Lett. 93, 108301-108304 (2004)
[3] R. Blumenfeld, Granular Matter 22, 38 (2020)
[4] M. Gerritsen, G. Kreiss, R. Blumenfeld, Phys. Rev. Lett. **101**, 098001 (2008)
[5] M. Gerritsen, G. Kreiss, R. Blumenfeld, Physica A **387**, 6263 (2008)
[6] R. Blumenfeld and J. Ma, J. Gran. Matt. 19:29 (2017)
